# Supplementary material for: QiMeng-CPU-v2: Automated Superscalar Processor Design by Learning Data Dependencies
Source: arXiv:2505.03195 source file (2025-05-06)
Supplement: Supplementary file 1 [file 8_appendix.tex]

\section{Preliminary: Circuit representation with BSDs}

%Based on BSD, it is possible to obtain the accurate Boolean functions of large-scale circuits only from input-output examples.

%BSD是什么
The BSD is a rooted, directed acyclic graph (DAG) that consists of internal decision nodes and leaf speculation nodes. The internal decision node indicates a Boolean variable with the assignment of value 0 or 1 to its two child nodes, and the speculation nodes approximate the sub-functions represented by the child nodes with constant 0 or 1.  

Therefore, the BSD is an efficient approximate representation of the combinational Boolean function. Since the precise representation of the sub-functions requires multiple nodes, the speculation nodes trade off the representation accuracy with a more compact structure. To decrease the accuracy loss, each speculation node in the BSD can be expanded with the Boole's Expansion Theorem into two child speculation nodes, formulated as follows: 
\begin{definition}[BSD Expansion]
\label{def:BSD expansion}
In the $k$-th expanding iteration, the sub-function represented by the speculation node $\mathcal{F}_k(\mathtt{x})$ can be represented with one less variable $x_i \in \mathtt{x}$, where $\mathtt{x}$ is the input variable set, $$\mathcal{F}_k(\mathtt{x})=\overline{x_i}\mathcal{F}_{k+1}(\mathtt{x}|x_i=0)+x_i\mathcal{F}_{k+1}(\mathtt{x}|x_i=1).$$
\end{definition}

It proved in the state-of-the-art paper~\cite{cheng2023pushing} that BSD expansion boosts the design accuracy of the combinational Boolean circuits, so that these combinational circuits can be functionally designed with only input-output examples, boosting the design accuracy with node expansion.
\begin{theorem}[The accuracy of BSD increases after node expansion]\label{thm:decomacc}
After expanding the generated BSD  $\mathcal{F}_k(\mathtt{x})$ (shorted as  $\mathcal{F}_k$) by any input bit $x_i$ to $\mathcal{F}_{k+1}$, the accuracy of expansion ended with $\mathcal{F}_k$ will be no larger than the accuracy of expansion ended with $\mathcal{F}_{k+1}$, that is, 
$$    Acc(\mathcal{F}_k) \leq  Acc(\mathcal{F}_{k+1}).$$

\end{theorem}

However, the BSD cannot design the sequential circuits in the same manner, because it cannot use the temporal information of the sequential circuits, which is not visible from the input-output example of the circuits. It fails to automatically design a superscalar processor.
